# Supplementary material for: SpaceEvo: Hardware-Friendly Search Space Design for Efficient INT8 Inference
Source: arXiv:2303.08308 source file (2023-03-15)
Supplement: Supplementary file 1 [file appendix.tex]

\newpage
\section{Experiment}
\label{sec:append_experiment}
\subsection{Experiment details}

\noindent\textbf{Supernet Training and QAT}. To train our quantized-for-all supernet, we perform two-stage training: (i) supernet pretraining without quantizers; and (ii) QAT on the pretrained supernet.  

\textit{(i) supernet pretraining without quantizers}. We use the sandwich rule and inplace distillation in BigNAS. Our training hyperparameters setting follows AlphaNet. Specifically, we use SGD with a cosine learning rate decay.  We train our supernet for 360 epochs on 8 Tesla Nvidia V100 GPUs. The mini-batch size is 128 per GPU. The initial learning rate is set as 0.1 and is linearly scaled up for every 256 training samples.
We use momentum of 0.9, weight decay of 1e-5, dropout of 0.2 after the global average pooling layer. We use AutoAugment for data augmentation and set label smoothing coefficient to 0.1. 

\textit{(ii) QAT on the pretrained supernet.} This step starts from a full-precision pretrained supernet. We load checkpoints from step (i) and perform LSQ+ for supernet quantization. The training receipt follows step (i) except we use a smaller learning rate of 0.01 and train the supernet for 50 epochs. 

\noindent\textbf{Quantization-aware NAS baselines}. In our paper, we focus on INT8 quantization because it has been widely supported on real-world devices. Since
existing quantization-aware NAS works focus on searching mixed-precision models, we would like not to directly compare our method with mixed-precision NAS works. We select the two state-of-the-art methods of APQ and OQAT and make some modifications based on their original settings.

APQ originally searches the model architecture and its layer-wise mixed-precision of \{4, 8\} bits. It manages an accuracy predictor that can predict the accuracy of a mixed-precision quantized model. To compare with APQ, we constrain each layer can only search 8bit. For fair comparison, we add our INT8 quantized latency predictor nn-Meter during the model search process. After the search finishes, we follow APQ to perform finetuning of 30 epochs. 

OQAT also trains a quantized-for-all supernet. However, it supports 4bit and 2 bit. To compare with OQAT, we simply modify its source code to quantize 8bit and re-do the supernet QAT process. Same with us, the supernet QAT is trained for 50 epochs. 

\subsection{Additional results}

\noindent\textbf{{\algname} under larger latency constraints for Intel CPU}. We provide additional results of search under larger latency constraints of \{10, 15, 20, 25, 30\}ms. The searched space structure is shown in Table~\ref{tbl:onnx_large}. We report the best searched quantized models and compare with {\algname}@CPU in Table~\ref{tbl:onnx_spacecompare}.  Under larger latency constraints,
the searched space  {\algname}@CPU-large produces better large models ($\geq$15 ms). 

\begin{table}[t]
	\centering
	%	\small
	\fontsize{8}{8} \selectfont
	\caption{ {\algname}@CPU-large: searched space under constraint of \{10, 15, 20, 25, 30\}ms. We report the best searched quantized model accuracy and latency.    }
	\begin{tabular}	%{@{\hspace{0.1\tabcolsep}}c@{\hspace{0.3\tabcolsep}}|@{\hspace{0.3\tabcolsep}}c@{\hspace{0.3\tabcolsep}}|@{\hspace{0.3\tabcolsep}}c@{\hspace{0.3\tabcolsep}}|@{\hspace{0.3\tabcolsep}}c@{\hspace{0.3\tabcolsep}}|@{\hspace{0.3\tabcolsep}}c@{\hspace{0.3\tabcolsep}}|@{\hspace{0.5\tabcolsep}}c@{\hspace{0.1\tabcolsep}}}
		{@{\hskip1pt}c@{\hskip1pt}|c@{\hskip1pt}@{\hskip2pt}c@{\hskip2pt}c@{\hskip1pt}c@{\hskip1pt}c@{\hskip1pt}c@{\hskip1pt}c@{\hskip1pt}}
		\hline
		\multirow{2}{*}{Search Space} & \multicolumn{6}{c}{Best searched models}\\
		& smallest & 8ms & 10ms & 15ms & 20ms & 25ms & 28ms \\
		\hline 
		{\algname}@CPU &74.7 (4.4ms) &76.7 &77.4 &78.7 &79.5&80.0 &80.1\\
		{\algname}@CPU-large  &76.2 (6.7ms) &76.5&77.1 &78.9 &79.7  &80.1 &80.3\\
		
		\hline
	\end{tabular}
	\label{tbl:onnx_spacecompare}
	
\end{table}

\begin{table}[t]
	%	\begin{adjustwidth}{-.12in}{-.1in}  
		\centering
		\fontsize{8}{8} \selectfont	
		\caption{ImageNet results compared with SOTA  quantized models on Pixel 6. $^*$: latency compared to FP32 inference.  }
		\begin{tabular}	
			{@{\hskip1pt}c|c|cc|c@{\hskip1pt}c@{\hskip1pt}}			
			\toprule
			\multicolumn{6}{c}{ \textbf{(b) Results on the Google Pixel 6 with TFLite}}\\
			\multirow{2}{*}{Model}  &Acc\%& \multicolumn{2}{c|}{Pixel4 Latency}&Acc\%& \multirow{2}{*}{FLOPs} \\
			&\textbf{ INT8}& \textbf{INT8}&\textbf{speedup$^*$} &   FP32&\\ 
			\midrule
			MobileNetV3Small & 66.3&3.7 ms & 1.4$\times$& 67.4 &56M \\
			OFA-pixel6& 73.9 & 5.1 ms &1.9$\times$ & 74.5& 165M\\
			\textbf{	\sysname @pixel6-A0}& \textbf{74.4} & \textbf{4.0 ms} & \textbf{2.2$\times$}  &74.5 & 112M \\
			\hline
			MobileNetV2  &71.4&9.5 ms  & 1.9$\times$&72.0&300M\\
			ProxylessNAS-R  &74.6 &9.9 ms &2.0$\times$&74.6&320M  \\
			
			MobileNetV3Large   &74.5&8.9 ms &1.6$\times$&75.2&219M \\
			OFA (\#25) &75.6&8.0 ms & 1.9$\times$&76.4 &230M\\
			OFA-pixel6& 76.2 & 10.1 ms &2.1$\times$ & 76.7& 337M\\
			AttentiveNAS-A0 &76.1 &8.7 ms  &2.2$\times$& 77.3& 203M \\
			\textbf{	\sysname @pixel6-A1}& \textbf{77.6} & \textbf{8.2 ms} & \textbf{2.4$\times$} & 77.7& 274M  \\
			\hline
			
			AttentiveNAS-A1&77.2&12.1 ms & 2.2$\times$&78.4&279M\\
			AttentiveNAS-A2&77.5&13.0 ms & 2.2$\times$ &78.8&317M\\		
			\textbf{	\sysname @pixel6-A2} & \textbf{78.3} & \textbf{11.2 ms} & \textbf{2.5$\times$} & 78.4& 412M\\
			\hline
			%	APQ-8bit && &75.5 & 30 ms & \\
			
			FBNetV2-L1 &75.8&14.0 ms &1.7$\times$&77.2& 325M \\
			OFA-pixel6& 76.7 & 14.8 ms &1.9$\times$ & 77.2& 403M\\
		
			FBNetV3-A  &78.2 &16.2 ms & 1.7$\times$& 79.1& 357M\\
		%	\textbf{	\sysname @pixel6-A4}  & \textbf{79.5} & \textbf{16.7 ms} & \textbf{2.4$\times$} & 79.5& 591M\\
			\textbf{	\sysname @pixel6-A3}  & \textbf{78.7} & \textbf{14.6 ms} & \textbf{2.5$\times$} & 78.8& 533M\\
			\hline
			EfficientNet-B0 &76.7&22.2 ms &1.7$\times$&77.3&390M \\
		%	\textbf{	\sysname @pixel6-A5}   & \textbf{79.9} & \textbf{20.2 ms} & \textbf{2.5$\times$} &80.0& 738M\\	
		\textbf{	\sysname @pixel6-A4}  & \textbf{79.6} & \textbf{19.5 ms} & \textbf{2.4$\times$} & 79.7& 676M\\
			\hline
		\end{tabular}		
		\label{tbl:endtoend}
	\end{table}
\noindent\textbf{Pixel 6 results.} We provide searched results on a new device. Specifically, we select Google Pixel 6 phone as our test device. We build INT8 quantized latency predictor with nn-Meter for Pixel 6. 
Table~\ref{tbl:endtoend} compares the searched quantized models performance with existing state-of-the-art efficient models and best-searched models from OFA MobileNetV3 search space (i.e., OFA-pixel6 in the Table). As we can see from Table~\ref{tbl:endtoend},  our searched space delivers significant better INT8 quantized models with higher accuracy and lower latency on Pixel 6 compared to those from OFA MobileNetV3 search space and existing state-of-the-art efficient models. For instance, SpaceEvo@pixel6-A0 runs 2.2$\times$ faster than MobileNetV3-Large with a same-level accuracy. SpaceEvo@pixel6-A4 achieves 79.6\% quantized accuracy on ImageNet with only 19.5ms, which is 2.7ms faster than EfficientNet-B0 with 2.9\% higher accuracy.  The searched quantized models achieve $\sim$2.4$\times$ latency speedup compared to FP32 inference, suggesting a better utilization of on-device INT8 quantization.

%\noindent\textit{Model distributions.} We first randomly sample quantized models from each search space to characterize the model error distributions~\cite{Radosavovic2019}. Specifically, we focus on comparing  low latency models and set two tight quantized latency constraints in  Fig.~\ref{fig:searchspace_quality}. Compared to SOTA search spaces,  we have significantly better model distributions in terms of quantized accuracy while under a same latency.  
%\begin{figure*}[t]
%	\centering
%	\includegraphics[width=0.8\textwidth]{figs/searchspace/modeldistribution/distribution1.png}	
%	\vspace{-2ex}
%	\caption{ Model error distribution comparison of different search spaces. For a target latency constraint on each device, we randomly sample 512 models from each search space and evaluate their quantized accuracy on ImageNet. }
%	\label{fig:searchspace_quality}
%\end{figure*}

\section{Block-wise quantization}
\textbf{NSR Loss}. For a sampled model block $m$ in the $i^{th}$ stage of a search space, it receives the output of the 
$(i-1)^{th}$ teacher block as the input and is optimized to predict the output of the  $i^{th}$ teacher block with NSR (per-channel noise-to-signal-power ratio) loss:

\begin{equation}
	\label{eq:nsrloss}
	\begin{aligned}
		\displaystyle \mathcal{L}({\mathop{E}(m)}^i, Y_i)= \frac{1}{C}\sum_{c=0}^{C}\frac{\|Y_{i,c}-f(Y_{i-1};{\mathop{E}(m)}^i)_c\|^2}{\sigma_{i,c}^2}
	\end{aligned}
\end{equation}
Where  ${\mathop{E}(m)}^i$  is a sampled block in elastic stage ${\mathop{E}}^i$, it take the  $(i-1)^{th}$ teacher block's output feature map $Y_{i-1}$ as the input.  $Y_i$ is the target output feature map of the $i^{th}$ block of the teacher model,   $f(Y_{i-1}; {\mathop{E}(m)}^i)$ maps the output feature map of the sampled block. $C$ is the number of channels in a feature map and $\sigma_{i,c}^2$ is the variance of $Y_{i,c}$.

\textbf{Training Hyperparameters}. All candidate elastic stages are trained in a parallel way. Specifically, each elastic stage is trained for 6 epochs on  4 V100 GPUs. The first 5 epochs are full-precision training. We use 0.005 as the initial learning rate for Stage 1 and Stage 6, and 0.01 for all the other Stages. We apply a cosine learning rate schedule, a batch size of 256, the Adam optimizer. After the full-precision training finishes, we conduct 1 epoch INT8 quantization-aware training with LSQ+. We use a much smaller learning rate of 0.0025 for quantization. 

\section{Device  and Latency Prediction }
\begin{table}[ht]
	\begin{center}
		%	\small
		\fontsize{8.2}{8.2} \selectfont
		
		\begin{tabular}	{@{\hspace{0.1\tabcolsep}}c@{\hspace{0.1\tabcolsep}}|@{\hspace{0.1\tabcolsep}}c@{\hspace{0.1\tabcolsep}}|@{\hspace{0.1\tabcolsep}}c@{\hspace{0.1\tabcolsep}}|@{\hspace{0.1\tabcolsep}}c@{\hspace{0.1\tabcolsep}}|@{\hspace{0.1\tabcolsep}}c@{\hspace{0.1\tabcolsep}}}
			\hline
			Name	 & Framework&Processor&Measured Hz& Precision\\
			\hline
			Intel VNNI &Onnxruntime v1.10 &\makecell{Intel (R) Xeon(R) \\Silver 4210 CPU} &2GHz &FP32/INT8 \\
			\hline
			Pixel 4 &TFLite v2.7 &CortexA76 CPU &2.42GHz & FP32/INT8\\
			\hline 
		\end{tabular}
		\caption{Our measured edge devices.  }
		\label{tbl:device}
	\end{center}
\end{table}

\begin{table}[ht]
	\begin{center}
		%	\small
		\fontsize{8.8}{8.8} \selectfont
		\begin{tabular}	{cccc}
			
			\toprule
		Device	&RMSE &$\pm$5\% accuracy & $\pm$10\% accuracy    \\
			\hline 
		Intel VNNI CPU &1.5ms&79.8\% & 92.5\%\\
		Pixel4 & 1.3ms & 89.6\%& 100\%\\
			\hline
		\end{tabular}
		\caption{INT8 quantized latency prediction performance of  nn-Meter. We report the $\pm$5\% and $\pm$10\% accuracy, that are the percentage
			of models with predicted latency within the corresponding error
			bound relative to the measured latency }
		\label{tbl:nnmeter}
	\end{center}
\end{table}

\begin{table}[t]
	\begin{center}
		%	\small
		\fontsize{8.5}{8.5} \selectfont
		
		\begin{tabular}	{c|cc|cc}
			\hline
			\multirow{2}{*}{
				\makecell{Kernel\\ size}}	& \multicolumn{2}{c|}{Intel VNNI CPU} & \multicolumn{2}{c}{Pixel4  }\\
			&Conv &DWConv   &Conv &DWConv  \\
			\hline 
			1 &3.5$\times$&2.7$\times$&2.6$\times$ &0.9$\times$  \\
			3 &3.6$\times$&1.4$\times$&4.0$\times$  &2.8$\times$\\
			5&3.8$\times$&1.1$\times$&3.9$\times$ &1.1$\times$ \\
			7&4.0$\times$&0.8$\times$ &3.8$\times$  &1.1$\times$ \\
			\hline
		\end{tabular}
		\caption{INT8 quantization speedup on two devices.  Kernel size impacts the speedup for DWConv.  Configuration: $H$=$W$=56, $C_{in}$=$C_{out}$=96.}
		\label{tbl:kernel_speedup}
	\end{center}
\end{table}

\noindent\textbf{Device details and latency measurement.} Table~\ref{tbl:device} lists out the detailed inference engine and hardware for our two measured devices. We select Intel VNNI CPU and Pixel 4 CPU because they support both FP32 and INT8 inference.  Specifically, we select TFLite and onnxruntime as the inference engines for Pixel 4 mobile CPU and Intel CPU, respectively, because they are well-known high-performance engines for edge AI inference. For latency measurement, we follow the practices in ~\cite{nnmeter,spacestudy,vitstudy}. We always measure the inference latency of a given model (either FP32 or INT8 quantized model) on a single CPU core with fixed frequency.  The inference batch size is 1. The reported latency in the paper is the arithmetic mean of 50 runs after 10 warmup runs. The 95\% confidence interval is within 2\%.

\noindent\textbf{Latency prediction of quantized models.} We now illustrate the details of building quantized latency predictors. Following the original nn-Meter paper, the latency of a given model is the sum of all kernels' predicted latency. Then the procedure contains two main steps: (i) detect kernels in a model, and (ii) build latency predictors for these kernels. For step (i), we perform the fusion rule detection in nn-Meter and detects 17 kernels (e.g., Conv-bn-relu and DWConv-bn-relu6). For step (ii),  we run the adaptive data sampler to collect training data for each kernel and train a randomforest regressor as the kernel-level latency predictor. Each training data sample is a pair of (configurations of a kernel, the inference latency). Taking Conv-bn-relu kernel as an example, we sample different kernel sizes, strides, input/output channel numbers and input resolution for Conv-bn-relu kernel, then we measure their INT8 quantized latency on the target device. 

The kernel-level latency predictors training and construction are conduct offline. During the evolutionary search, we use them to predict the INT8 quantized latency for arbitrary model. Table~\ref{tbl:nnmeter} lists out the prediction performance. Specifically, we randomly sample 2k models and predict their INT8 quantized latency  for evaluation. Remarkably, nn-Meter achieves   92.5\% and 100\% prediction accuracy on the Intel VNNI CPU and Pixel 4, respectively.

\section{Additional Quantization Efficiency Analysis}
\label{sec:channels}

\begin{figure}[th]
	\centering
	\includegraphics[width=1.1\columnwidth]{figs/data/dwconv_channel.png}	
	
	\caption{The choice of channel number greatly impact the INT8 latency of DWConv.   INT8 latency of DWConv shows a step pattern.  Configuration: $HW$=28. We set a large DWConv channel number for measurement because expansion ratios are usually larger than 3.  }
	
	\label{fig:dwconvchannel}
\end{figure}

In Section 2, we studied how the operator type and channel widths in a quantized model impact final inference efficiency. Next, we will illustrate the impact of other configuration dimensions.

\noindent\textbf{Kernel size.} Table~\ref{tbl:kernel_speedup} shows the latency speedup of Conv and DWConv with different kernel sizes. Results suggest that the choice of kernel size can result in different speedups after INT8 quantization. Specifically, we notice that kernel size is more crucial to DWConv quantization efficiency than Conv. Unlike Conv can consistently achieve speedups under various kernel sizes, improper kernel size of DWConv can lead to a significant slowdown. Moreover, the most efficient kernel size for DWConv is highly relying on the target devices. DWConv with smaller kernel sizes can achieve larger speedup on Intel CPU, while DWConv with $K=3$ achieves the maximum speedup of 2.8$\times$ on Pixel 4. 

Consequently, the INT8 quantized models should consider the choices of kernel sizes to achieve both high accuracy and low inference latency. Instead of searching the optimal kernel sizes for a search space, we directly allow all stages  to choose from \{3, 5, 7\}. In our work, we perform latency-aware evolutionary search to derive the optimal quantized models from the resulting search space.  As shown in Table~\ref{tbl:onnx_seqnet} and Table~\ref{tbl:pixel4_seqnet}, the optimal quantization-friendly kernel sizes are chosen for our discovered model family {\sysname}.  For example, kernel size of 3$\times$3 is the dominate choice in DWConv in {\sysname}.

\noindent\textbf{Channel number of DWConv.}	Fig.~\ref{fig:dwconvchannel}  show the latency of DWConv 3$\times$3 with different channel number on two devices. Surprisingly, we observe a step pattern: the latency of DWConv 3$\times$3 achieves minimal at special channel numbers. Specifically,  in terms of INT8 quantized latency, 
when $C$ is divisible to 8 on Pixel 4 (16 on Intel CPU), the latency achieves a minimal and can be accelerated by 2.9$\times$ ( 1.7$\times$ on Intel CPU). Therefore, we constrain the channel widths in our search space to be divisible by 8 on Pixel 4 and 16 on Intel CPU.  Moreover, we notice that the latency patterns of FP32 and INT8 inference are different on two devices, which further motivates {\algname}.

\section{Search Space Design Details}

\begin{table}[ht]
		\begin{minipage}[b]{0.48\textwidth}
			\centering
			%	\small
			\fontsize{8.2}{8.2} \selectfont
			
			\begin{tabular}	{@{\hspace{0.1\tabcolsep}}c@{\hspace{0.3\tabcolsep}}|@{\hspace{0.3\tabcolsep}}c@{\hspace{0.3\tabcolsep}}|@{\hspace{0.3\tabcolsep}}c@{\hspace{0.3\tabcolsep}}|@{\hspace{0.3\tabcolsep}}c@{\hspace{0.3\tabcolsep}}|@{\hspace{0.3\tabcolsep}}c@{\hspace{0.3\tabcolsep}}|@{\hspace{0.5\tabcolsep}}c@{\hspace{0.5\tabcolsep}}}
				\hline
				Stage	 & Depths & \makecell{Kernel\\ Size}&Stride& \makecell{Channel\\ Widths \\ 16-divisible} & ck\\
				
				\hline 
				Conv (STEM)& 1 & 3  & 2  & 16 - 32 & - \\
				Residual (STEM) &1-2&3  & 1 & 16 - 32& -\\
				Stage1&2-4&3, 5, 7&2&32 - 64&2\\
				Stage2&2-4&3, 5, 7&2&32 - 96&2\\
				Stage3&2-6&3, 5, 7&2&64 - 144&3\\
				Stage4&2-6&3, 5, 7&1&112 - 192&3\\
				Stage5&2-6&3, 5, 7&2&192 - 304&5\\
				Stage6&1-2&3, 5, 7&1&304 - 448&7\\
				Classifier (head)&-&-&-&-&-\\
				\hline 
				input resolution& \multicolumn{5}{c}{160, 176, 192, 208, 224}\\
				
				\hline
			\end{tabular}
			
			\caption{CPU hyperspace. We search the optimal block type and channel widths for Stage1-6.  }
			\label{tbl:hyperspaceonnx}
			
		\end{minipage}
		\hfill \hfill
		\begin{minipage}[b]{0.49\textwidth}
		\centering
				%	\small
				\fontsize{8.2}{8.2} \selectfont
			
				\begin{tabular}	{@{\hspace{0.1\tabcolsep}}c@{\hspace{0.3\tabcolsep}}|@{\hspace{0.3\tabcolsep}}c@{\hspace{0.3\tabcolsep}}|@{\hspace{0.3\tabcolsep}}c@{\hspace{0.3\tabcolsep}}|@{\hspace{0.3\tabcolsep}}c@{\hspace{0.3\tabcolsep}}|@{\hspace{0.3\tabcolsep}}c@{\hspace{0.3\tabcolsep}}|@{\hspace{0.5\tabcolsep}}c@{\hspace{0.5\tabcolsep}}}
					\hline
					Stage	 & Depths &\makecell{ Kernel \\Size}&Stride& \makecell{Channel\\ Widths \\ 8-divisible} & ck\\
					
					\hline 
					Conv (STEM)& 1 & 3  & 2  & 16-32 & - \\
					MBv2 (STEM) &1-2&3  & 1 & 16-32& -\\
					Stage1&2-4&3, 5, 7&2&24 - 32&2\\
					Stage2&2-6&3, 5, 7&2&40 - 56&2\\
					Stage3&2-6&3, 5, 7&2&80 - 104&3\\
					Stage4&2-8&3, 5, 7&1&96 - 128&3\\
					Stage5&2-8&3, 5, 7&2&192 - 256&5\\
					Stage6&1-2&3, 5, 7&1&320 - 416&7\\
					Classifier (head)&-&-&-&-&-\\
					\hline 
					input resolution& \multicolumn{5}{c}{160, 176, 192, 208, 224}\\

					\hline
				\end{tabular}
				
	\caption{Pixel4 hyperspace. We search the optimal block type and channel widths for Stage1-6.  }
\label{tbl:hyperspacepixel4}
			
				\end{minipage}
\end{table}

\begin{table*}[ht]

			\centering
			%	\small
			\fontsize{8.2}{8.2} \selectfont
			
			\begin{tabular}	%{@{\hspace{0.1\tabcolsep}}c@{\hspace{0.1\tabcolsep}}|@{\hspace{0.1\tabcolsep}}c@{\hspace{0.1\tabcolsep}}|@{\hspace{0.1\tabcolsep}}c@{\hspace{0.1\tabcolsep}}|@{\hspace{0.5\tabcolsep}}c@{\hspace{0.5\tabcolsep}}}
				{c|c|cc|cc}
				\hline
				\multirow{2}{*}{Block type}&	\multirow{2}{*}{Search id}	 &\multicolumn{2}{c|}{Intel CPU}&\multicolumn{2}{c}{Pixel4} \\
				& & Expand Ratios & Activation & Expand Ratios & Activation\\
				
				\hline 
				MBv1&0&- & relu &- & relu\\
				MBv2&1&4, 6, 8 & relu6&3, 6, 8 & relu6 \\
				MBv3& 2&4, 6, 8& hswish & 3, 6, 8& swish\\
				Residual bottleneck &3& 0.5, 1.0, 1.5 & relu& 0.5, 1.0, 1.5 & relu \\
				Residual bottleneck+SE &4& 0.5, 1.0, 1.5 & relu& 0.5, 1.0, 1.5 & relu \\
				FusedMB & 5&1, 2, 3, 4 & swish  & 1, 2, 3, 4 & swish \\
				FusedMB+SE &6& 1, 2, 3, 4 & swish& 1, 2, 3, 4 & swish  \\

				\hline
			\end{tabular}
			\caption{Block choices for an elastic stage. We set larger expand ratios and use swish as the activation function  }
			\label{tbl:hyperspaceonnx_1}
	
\end{table*}
 
\noindent\textbf{Hyperspace}. Table~\ref{tbl:hyperspaceonnx} and Table~\ref{tbl:hyperspacepixel4} summarize the hyperspace structures when targeting Intel VNNI CPU and Pixel 4 mobile CPU, respectively. As introduced in Section 3, we search the 6 stages (Stage1-Stage6) for a quantization-friendly search space. For each elastic stage, it can search: (i) an optimal block type from a pool as shown in Table~\ref{tbl:hyperspaceonnx_1}; and (ii) the optimal channel widths for that block type as shown in Table~\ref{tbl:hyperspaceonnx} and Table~\ref{tbl:hyperspacepixel4}. Other search space dimensions including kernel sizes, expand ratios and input resolutions are unsearchable and using manual settings.  
 
In total, the hyperspace contains $\sim$10$^9$ possible candidate search spaces, which is extremely large and we leverage the aging evolution for efficient search. For better mutations, we encode a candidate search space as the format of \textit{PerStageBlock}-\textit{PerStageWidth}. As shown in Table~\ref{tbl:hyperspaceonnx_1}, we assign an unique search id for each candidate block types. For example, 1 indicates selecting the MBv2 block.  For the channel widths, we use the minimal channel index as the encoding. For example, 0 indicates selecting channel widths of \{32, 48\} (32 is the $0^{th}$ item in \{32, 48, 64\}) for Stage1 on the Intel CPU; 1 indicates selecting \{48, 64\}.  
Taking 111111-000000 as an example, it means that all stages choose the MBv2 block; and the chosen channel widths for Stage1 to Stage6 are \{32, 48\}, \{32, 48\},  \{64, 80, 96\},  \{112, 128, 144\},  \{192, 208, 224, 240, 256\},  \{304, 320, 336, 352, 368, 384, 400\}, respectively.

%\begin{figure}[th]
%	\centering
%	\includegraphics[width=0.9\columnwidth]{figs/pipeline.png}	
	
%	\caption{Our overall pipeline has three steps: search a quantization-friendly search space; train a quantized-for-all supernet; search an optimal quantized model under diverse latency constraints. }
	
%	\label{fig:pipeline}
%\end{figure}

\algrenewcommand{\algorithmiccomment}[1]{$\triangleright$ #1}
\begin{algorithm}[h]
	\small
	\caption{Search Space Evolution Algorithm}\label{alg}
	\label{alg:spacesearch}
	\begin{flushleft}
		\textbf{Input}: Hyperspace $\mathcal{H}$, 
		total number of spaces to explore $N$, population size $P$, sample \\size $S$, latency\_auc tradeoff $\alpha$, target latency constraints $T_{0,1,..n}$\\
		%\yh{should we make $S$ and $P$ the same since it is the same in our experiments?}
		
		%	\textbf{Output}: optimal layer-wise sparsity 
	\end{flushleft}
	\begin{algorithmic}[1]		
		\State $population^{(0)}$ $\gets$ \texttt{initialize} ($\mathcal{H}$, $P$)

		\For{$i$=1: ($N$-$P$)}
		\State $parent$ $\gets$ \texttt{sample\_with\_maximum\_score} ($population^{(i-1)}$,$S$)
		\State $child_1$ $\gets$ \texttt{mutate-block-type} ($parent$, $T_{0,1,..n}$)
		\State $score_1$ $\gets$ \texttt{get\_quality\_score} ($child_1$, $T_{0,1,..n}$,$\alpha$ ) (see Equation 2)
		\State $child_2$ $\gets$ \texttt{mutate-block-width} ($parent$, $T_{0,1,..n}$)
		\State $score_2$ $\gets$ \texttt{get\_quality\_score} ($child_2$, $T_{0,1,..n}$, $\alpha$ ) (see Equation 2)
		
		\State $population^{(i)}$$\gets$ add $child_1$ and $child_2$ to right of $population^{(i-1)}$, remove the oldest two spaces from left of  $population^{(i-1)}$
		\EndFor
		\State return the search space with maximum score under the $T_{0,1,...n}$
	\end{algorithmic}
\end{algorithm}

\noindent\textbf{Search algorithm.} Algorithm~\ref{alg:spacesearch} illustrates the major procedures of searching a quantization-friendly search space. To generate the initial population, we randomly sample $P$=500 search spaces from the hyperspace, then we perform random mutations to evolve better search spaces. Specifically, for each evolution iteration, we first sample $S$=125 spaces from the current population, and select the one with highest Q-T score as the parent. Then we alternately mutate the parent and produce two children (line 4-7). The following illustrates an example. 
Assume the search space 111111-000000 is selected as the parent, and  stage 2 is randomly selected for mutation. For the block type mutation, 
an example child$_1$ 131111-000000 is produced. For the channel width mutation, we can randomly create 111111-020000 as the child$_2$. We add the two children into the current population and remove the oldest two for next iteration. In total, we search 5k search spaces for each device.

 Fig.~\ref{fig:searchalgorithm} compares the search efficiency with random search.  For each method, we set a same range of latency constraints, and keep track of the searched spaces for every 500 iterations. We select the top 10 spaces with the best Q-T score over time.  Fig.~\ref{fig:searchalgorithm} demonstrates that our space evolution algorithms consistently achieve better search spaces (i.e., higher Q-T score) than random search. 
\begin{figure}
	\centering
	\includegraphics[width=1\columnwidth]{figs/searchspace/searchalgorithm/searchalgorithm.png}	
	\caption{Space search efficiency comparison. }
	\label{fig:searchalgorithm}
\end{figure}

\section{Architecture visualization of {\sysname}}
We visualize the searched INT8 quantized model architectures in Table~\ref{tbl:onnx_seqnet} and Table~\ref{tbl:pixel4_seqnet}. ‘d’ denotes number of layers, ‘c’ denotes the number of output channels, ‘k’ denotes
kernel size, ‘e’ denotes expansion ratio.  If a stage has multiple layers, we list out the kernel size, output channel numbers, expansion ratios for each layer and use ‘-’to separate them. For example, c: 32-48 indicates that the channel numbers are 32 for the first layer and 48 for the second layer.  

\begin{table*}[t]
	\centering
	\fontsize{8.2}{8.2} \selectfont	
	\begin{tabular}
			{@{\hspace{0.1\tabcolsep}}c@{\hspace{0.5\tabcolsep}}|@{\hspace{0.5\tabcolsep}}c@{\hspace{0.5\tabcolsep}}|@{\hspace{0.5\tabcolsep}}c@{\hspace{0.5\tabcolsep}}|@{\hspace{0.5\tabcolsep}}c@{\hspace{0.5\tabcolsep}}|@{\hspace{0.5\tabcolsep}}c@{\hspace{0.5\tabcolsep}}|@{\hspace{0.5\tabcolsep}}c@{\hspace{0.1\tabcolsep}}}
			\hline
	 & {\sysname}@cpu-A0 &{\sysname}@cpu-A1 & {\sysname}@cpu-A2& {\sysname}@cpu-A3& {\sysname}@cpu-A4  \\
		\hline 
	
		Conv &\makecell{d: 1\\c: 16\\k: 3 } &\makecell{d: 1\\c: 16\\k: 3 }&\makecell{d: 1\\c: 16\\k: 3 } & \makecell{d: 1\\c: 16\\k: 3 } &\makecell{d: 1\\c: 32\\k: 3 }   \\
		\hline
		Residual bottleneck &\makecell{d: 1\\c: 16\\k: 3 \\e: 0.5 } &\makecell{d: 1\\c: 16\\k: 3 \\e: 0.5 }&\makecell{d: 1\\c: 16\\k: 3 \\e: 0.5 }  &\makecell{d: 1\\c: 32\\k: 3 \\e: 0.5 } & \makecell{d: 1\\c: 32\\k: 3 \\e: 0.5 }\\
		\hline
		MBv2 & \makecell{d: 2\\c: 32-32\\k: 3-3\\e: 4-4  }&\makecell{d: 2\\c: 32-32\\k: 3-3\\e: 4-4  } &\makecell{d: 2\\c: 32-32\\k: 3-3\\e: 4-6  } &\makecell{d: 2\\c: 32-48\\k: 3-3\\e: 4-8  } & \makecell{d: 3\\k: 3-3-3\\c: 48-48-32\\e: 4-6-6 }\\
		\hline
		FusedMB &\makecell{d: 2\\c: 64-64\\k: 3-3\\e: 1-1 } &\makecell{d: 2\\c: 64-80\\k: 3-3\\e: 2-1 } &\makecell{d: 2\\c: 64-64\\k: 3-3\\e: 3-2 } &\makecell{d: 2\\c: 80-80\\k: 3-3\\e: 4-2 } & \makecell{d: 3\\c: 64-64-64\\k: 5-3-3\\e: 4-3-1}\\
		\hline
		MBv2 & \makecell{d: 2\\c: 112-112\\k: 3-3\\e: 4-4 }&  \makecell{d: 3\\c: 128-112-112\\k: 3-5-3\\e: 4-6-4 }&  \makecell{d: 4\\c: 112-112-128\\k: 3-3-5-5\\e: 4-4-6-8 }&\makecell{d: 3\\c: 144-128-112\\k: 5-5-5\\e: 6-6-6 } &\makecell{d: 4\\c: 112-112-112-112\\k: 5-5-3-5\\e: 8-8-4-4} \\
		\hline
		MBv2 &\makecell{d: 2\\c: 144-144\\k: 3-3\\e: 4-4 } &\makecell{d: 2\\c: 144-176\\k: 3-3\\e: 4-4 }  &\makecell{d: 4\\c: 144-144-160-160\\k: 3-5-5-3\\e: 8-4-4-4 } & \makecell{d: 4\\c: 144-176-144-144\\k: 3-3-5-3\\e: 6-8-4-4 } & \makecell{d: 5\\c: 176-176-144-144-160\\k: 5-5-3-3-3\\e: 8-4-4-6-4 }  \\
		\hline
		MBv3 (hswish) & \makecell{d: 2\\c: 240-240\\k: 3-3\\e: 4-4  }&\makecell{d: 3\\c: 304-304-256\\k: 3-3-3\\e: 4-6-4  }&\makecell{d: 4\\c: 288-272-288-256\\k: 3-3-3-3\\e: 4-6-6-4  } &\makecell{d: 4\\c: 272-288-272-240\\k: 3-5-3-3\\e: 8-6-4-6  } & \makecell{d: 4\\c: 304-272-272-288\\k: 3-3-5-3\\e: 8-8-6-4  }\\
		\hline
		MBv3 (hswish) &\makecell{d: 1\\c: 320\\k: 3\\e: 4 } &\makecell{d: 1\\c: 368\\k: 5\\e: 4 } &\makecell{d: 1\\c: 320\\k: 5\\e: 4 } & \makecell{d: 1\\c: 320\\k: 3\\e: 6 } &\makecell{d: 2\\c: 352-320\\k: 3-3\\e: 6-4 }  \\
		\hline
		Resolution &160 &192 &208&224 & 224\\
		\hline
	\end{tabular}
	
	\caption{  INT8 quantized models produced by {\algname}@CPU.  }
	\label{tbl:onnx_seqnet}	
\end{table*}

\begin{table*}[t]
	\centering
	\fontsize{8.2}{8.2} \selectfont
	\begin{tabular}	
		{@{\hspace{0.1\tabcolsep}}c@{\hspace{0.5\tabcolsep}}|@{\hspace{0.5\tabcolsep}}c@{\hspace{0.5\tabcolsep}}|@{\hspace{0.5\tabcolsep}}c@{\hspace{0.5\tabcolsep}}|@{\hspace{0.5\tabcolsep}}c@{\hspace{0.5\tabcolsep}}|@{\hspace{0.5\tabcolsep}}c@{\hspace{0.5\tabcolsep}}|@{\hspace{0.5\tabcolsep}}c@{\hspace{0.1\tabcolsep}}}
		\hline
		& {\sysname}@pixel4-A0 &{\sysname}@pixel4-A1 & {\sysname}@pixel4-A2& {\sysname}@pixel4-A3& {\sysname}@pixel4-A4  \\
		\hline 
		
		Conv &\makecell{d: 1\\c: 16\\k: 3 } &\makecell{d: 1\\c: 16\\k: 3 }&\makecell{d: 1\\c: 16\\k: 3 } & \makecell{d: 1\\c: 16\\k: 3 } &\makecell{d: 1\\c: 24\\k: 3 }   \\
		\hline
		MBv2 &\makecell{d: 1\\c: 16\\k: 3 \\e: 1} &\makecell{d: 1\\c: 16\\k: 3 \\e: 1 }&\makecell{d: 1\\c: 16\\k: 3 \\e: 1 }  &\makecell{d: 1\\c: 16\\k: 3 \\e: 1 } & \makecell{d: 2\\c: 16-24\\k: 3-3 \\e: 1-1 }\\
		\hline
		MBv2 & \makecell{d: 2\\c: 32-32\\k: 3-3\\e: 3-3  }&\makecell{d: 2\\c: 32-32\\k: 3-3\\e: 3-3  } &\makecell{d: 2\\c: 40-32\\k: 3-3\\e: 3-3  } &\makecell{d: 2\\c: 32-32\\k: 3-3\\e: 8-3  } & \makecell{d: 2\\k: 3-3\\c: 32-32\\e: 6-8  }\\
		\hline
		MBv3 &\makecell{d: 2\\c: 64-64\\k: 3-3\\e: 3-3 } &\makecell{d: 2\\c: 64-64\\k: 3-3\\e: 3-3 } &\makecell{d: 2\\c: 64-72\\k: 3-3\\e: 3-3 } &\makecell{d: 3\\c: 64-72\\k: 3-3-5\\e: 3-6-3 } & \makecell{d: 3\\c: 72-64-64\\k: 3-3-5\\e: 6-3-3}\\
		\hline
		MBv3 & \makecell{d: 2\\c: 96-96\\k: 3-3\\e: 3-3 }&  \makecell{d: 2\\c: 96-96\\k: 7-3\\e: 3-3 }&  \makecell{d: 2 \\c: 96-96\\k: 3-3\\e: 3-6 }&\makecell{d: 3\\c: 64-112-96\\k: 7-3-3\\e: 8-3-6 } &\makecell{d: 4\\c: 112-96-104-104\\k: 3-5-5-3\\e: 6-6-3-3} \\
		\hline
		MBv3 &\makecell{d: 2\\c: 144-144\\k: 3-3\\e: 3-3 } &\makecell{d: 2\\c: 144-144\\k: 3-3\\e: 3-3 }  &\makecell{d: 3\\c: 152-160-152\\k: 5-3-3\\e: 3-6-3} & \makecell{d: 4\\c: 104-152-144-152\\k: 3-3-3-5\\e: 6-6-3-3 } & \makecell{d: 4\\c: 152-144-144-152\\k: 3-3-3-5\\e: 8-8-6-3 }  \\
		\hline
		MBv3 & \makecell{d: 2\\c: 192-192\\k: 3-3\\e: 3-3  }&\makecell{d: 4\\c: 224-192-208-192\\k: 3-3-5-3\\e: 6-6-6-3  }&\makecell{d: 4\\c: 200-224-200-200\\k: 7-5-7-5\\e: 6-3-3-6  } &\makecell{d: 4\\c: 200-192-208-192\\k: 3-3-3-5\\e: 6-8-6-6  } & \makecell{d: 5\\c: 224-216-208-224-208\\k: 7-5-3-5-3\\e: 8-6-6-3-3  }\\
		\hline
		MBv3 &\makecell{d: 1\\c: 216\\k: 3\\e: 3 } &\makecell{d: 1\\c: 232\\k: 3\\e: 3 } &\makecell{d: 1\\c: 248\\k: 5\\e: 3 } & \makecell{d: 1\\c: 280\\k: 3\\e: 6 } &\makecell{d: 1\\c: 296\\k: 3\\e: 6 }  \\
		\hline
		Resolution &160 &208 &224&224 & 224\\
		\hline
	\end{tabular}	
	\caption{INT8 quantized models produced by {\algname}@Pixel4 }
	\label{tbl:pixel4_seqnet}	
\end{table*}

\section{Searched space}
 Table~\ref{tbl:onnxspace} and Table~\ref{tbl:pixel4} list out the searched space structures for Intel CPU and Pixel4 mobile CPU, respectively.
In experiment section, the main results (are reported through searching the two search spaces. In addition, we provide 
the detailed search space structures under other latency constraints in Table~\ref{tbl:pixel4_medium}, Table~\ref{tbl:pixel4_small}  and Table~\ref{tbl:onnx_large}.
\begin{table*}[t]
	\centering
	\fontsize{8.2}{8.2} \selectfont
		\caption{{\algname}@CPU: searched space under constraint of \{8, 10, 15, 20, 25\}ms on CPU.   }
	\label{tbl:onnxspace}	
	\begin{tabular}	{@{\hspace{0.1\tabcolsep}}c@{\hspace{0.3\tabcolsep}}|@{\hspace{0.3\tabcolsep}}c@{\hspace{0.3\tabcolsep}}|@{\hspace{0.3\tabcolsep}}c@{\hspace{0.3\tabcolsep}}|@{\hspace{0.3\tabcolsep}}c@{\hspace{0.3\tabcolsep}}|@{\hspace{0.3\tabcolsep}}c@{\hspace{0.3\tabcolsep}}|@{\hspace{0.5\tabcolsep}}c@{\hspace{0.1\tabcolsep}}}
		\hline
		Stage	 & Depths & \makecell{Kernel\\ Size}&Stride& \makecell{Channel\\ Widths \\ 16-divisible} & \makecell{Expand\\ Ratio}\\		
		\hline 
		Conv & 1 & 3  & 2  & 16 - 32 & - \\
		Residual bottleneck &1-2&3  & 1 & 16 - 32& 0.5\\
		MBv2&2-4&3, 5, 7&2&32 - 48&4, 6, 8\\
		FusedMB&2-4&3, 5, 7&2&64 - 80&1, 2, 3, 4\\
		MBv2&2-6&3, 5, 7&2&112 - 144&4, 6, 8\\
		MBv2&2-6&3, 5, 7&1&144 - 176&4, 6, 8\\
		MBv3 (hswish)&2-6&3, 5, 7&2&240 -304&4, 6, 8\\
		MBv3 (hswish)&1-2&3, 5, 7&1&320 - 416&4, 6, 8\\
		Classifier&-&-&-&-&-\\
		\hline 
		input resolution& \multicolumn{5}{c}{160, 176, 192, 208, 224}\\	
		\hline
	\end{tabular}	

\end{table*}
\begin{table*}[t]
	\centering
	\fontsize{8.2}{8.2} \selectfont	
		\caption{{\algname}@Pixel4: searched space under constraint of \{15, 20, 25, 30, 35\}ms on Pixel4.  }
	\label{tbl:pixel4}		
	\begin{tabular}	{@{\hspace{0.1\tabcolsep}}c@{\hspace{0.3\tabcolsep}}|@{\hspace{0.3\tabcolsep}}c@{\hspace{0.3\tabcolsep}}|@{\hspace{0.3\tabcolsep}}c@{\hspace{0.3\tabcolsep}}|@{\hspace{0.3\tabcolsep}}c@{\hspace{0.3\tabcolsep}}|@{\hspace{0.3\tabcolsep}}c@{\hspace{0.3\tabcolsep}}|@{\hspace{0.5\tabcolsep}}c@{\hspace{0.1\tabcolsep}}}
		\hline
		Stage	 & Depths &\makecell{ Kernel \\Size}&Stride& \makecell{Channel\\ Widths \\ 8-divisible} & \makecell{Expand\\ Ratio}\\		
		\hline 
		Conv & 1 & 3  & 2  & 16-32 & - \\
		MBv2  &1-2&3  & 1 & 16-32& 1\\
		MBv2&2-4&3, 5, 7&2&32 - 40&3, 6, 8\\
		MBv3&2-6&3, 5, 7&2&64 - 72&3, 6, 8\\
		MBv3&2-6&3, 5, 7&2&96 - 112&3, 6, 8\\
		MBv3&2-8&3, 5, 7&1&144 - 160&3, 6, 8\\
		MBv3&2-8&3, 5, 7&2&192 - 224&3, 6, 8\\
		MBv3&1-2&3, 5, 7&1&216 - 312&3, 6, 8\\
		Classifier&-&-&-&-&-\\
		\hline 
		input resolution& \multicolumn{5}{c}{160, 176, 192, 208, 224}\\			
		\hline
	\end{tabular}	

\end{table*}

\begin{table*}[t]
	\centering
	\fontsize{8.2}{8.2} \selectfont	
		\caption{{\algname}@Pixel4-medium: searched space under constraint of \{10, 15, 20, 25, 30\}ms.   }
	\label{tbl:pixel4_medium}
	\begin{tabular}	{@{\hspace{0.1\tabcolsep}}c@{\hspace{0.3\tabcolsep}}|@{\hspace{0.3\tabcolsep}}c@{\hspace{0.3\tabcolsep}}|@{\hspace{0.3\tabcolsep}}c@{\hspace{0.3\tabcolsep}}|@{\hspace{0.3\tabcolsep}}c@{\hspace{0.3\tabcolsep}}|@{\hspace{0.3\tabcolsep}}c@{\hspace{0.3\tabcolsep}}|@{\hspace{0.5\tabcolsep}}c@{\hspace{0.1\tabcolsep}}}
		\hline
		Stage	 & Depths & \makecell{Kernel\\ Size}&Stride& \makecell{Channel\\ Widths \\ 8-divisible} & \makecell{Expand\\ Ratio}\\	
		\hline 
		Conv & 1 & 3  & 2  & 16 - 32 & - \\
		MBv2 &1-2&3  & 1 & 16 - 32& 1\\
		MBv2&2-4&3, 5, 7&2&32 - 40&3, 6, 8\\
		MBv2&2-4&3, 5, 7&2&64 - 72&3, 6, 8\\
		MBv3&2-6&3, 5, 7&2&88 - 104&3, 6, 8\\
		MBv3&2-6&3, 5, 7&1&144 - 160&3, 6, 8\\
		MBv3&2-6&3, 5, 7&2&200 - 240&3, 6, 8\\
		MBv1&1-2&3, 5, 7&1&216 - 312&3, 6, 8\\
		Classifier&-&-&-&-&-\\
		\hline 
		input resolution& \multicolumn{5}{c}{160, 176, 192, 208, 224}\\	
		\hline
	\end{tabular}

\end{table*}

\begin{table*}[t]
	\centering
	\fontsize{8.2}{8.2} \selectfont	
	\caption{{\algname}@Pixel4-tiny: searched space under constraint of \{6, 10, 15, 20, 25\}ms.  }
	\label{tbl:pixel4_small}	
	\begin{tabular}	{@{\hspace{0.1\tabcolsep}}c@{\hspace{0.3\tabcolsep}}|@{\hspace{0.3\tabcolsep}}c@{\hspace{0.3\tabcolsep}}|@{\hspace{0.3\tabcolsep}}c@{\hspace{0.3\tabcolsep}}|@{\hspace{0.3\tabcolsep}}c@{\hspace{0.3\tabcolsep}}|@{\hspace{0.3\tabcolsep}}c@{\hspace{0.3\tabcolsep}}|@{\hspace{0.5\tabcolsep}}c@{\hspace{0.1\tabcolsep}}}
		\hline
		Stage	 & Depths &\makecell{ Kernel \\Size}&Stride& \makecell{Channel\\ Widths \\ 8-divisible} & \makecell{Expand\\ Ratio}\\
		\hline 
		Conv & 1 & 3  & 2  & 16-32 & - \\
		MBv2  &1-2&3  & 1 & 16-32& 1\\
		Residual bottleneck&2-4&3, 5, 7&2&32 - 40&3, 6, 8\\
		Residual bottleneck&2-6&3, 5, 7&2&48 - 56&3, 6, 8\\
		MBv3&2-6&3, 5, 7&2&88- 104&3, 6, 8\\
		MBv2&2-8&3, 5, 7&1&128 - 144&3, 6, 8\\
		MBv2&2-8&3, 5, 7&2&192 - 224&3, 6, 8\\
		MBv1&1-2&3, 5, 7&1&216 - 312&3, 6, 8\\
		Classifier&-&-&-&-&-\\
		\hline 
		input resolution& \multicolumn{5}{c}{160, 176, 192, 208, 224}\\
		\hline
	\end{tabular}	
	
\end{table*}

\begin{table*}[t]
	\centering
	\fontsize{8.2}{8.2} \selectfont
	\caption{{\algname}@CPU-large: searched space under constraint of \{10, 15, 20, 25, 30\}ms.  }
	\label{tbl:onnx_large}	
	\begin{tabular}	
		{@{\hspace{0.1\tabcolsep}}c@{\hspace{0.3\tabcolsep}}|@{\hspace{0.3\tabcolsep}}c@{\hspace{0.3\tabcolsep}}|@{\hspace{0.3\tabcolsep}}c@{\hspace{0.3\tabcolsep}}|@{\hspace{0.3\tabcolsep}}c@{\hspace{0.3\tabcolsep}}|@{\hspace{0.3\tabcolsep}}c@{\hspace{0.3\tabcolsep}}|@{\hspace{0.5\tabcolsep}}c@{\hspace{0.1\tabcolsep}}}
		\hline
		Stage	 & Depths & \makecell{Kernel\\ Size}&Stride& \makecell{Channel\\ Widths \\ 16-divisible} & \makecell{Expand\\ Ratio}\\
		
		\hline 
		Conv & 1 & 3  & 2  & 16 - 32 & - \\
		Residual bottleneck &1-2&3  & 1 & 16 - 32& 0.5\\
		MBv2&2-4&3, 5, 7&2&48 - 64&4, 6, 8\\
		MBv3 (hswish)&2-4&3, 5, 7&2&80 - 96&4, 6, 8\\
		MBv2&2-6&3, 5, 7&2&112 - 144&4, 6, 8\\
		MBv2&2-6&3, 5, 7&1&160 - 192&4, 6, 8\\
		MBv3 (hswish)&2-6&3, 5, 7&2&240 - 304&4, 6, 8\\
		MBv3 (hswish)&1-2&3, 5, 7&1&320 - 416&4, 6, 8\\
		Classifier&-&-&-&-&-\\
		\hline 
		input resolution& \multicolumn{5}{c}{160, 176, 192, 208, 224}\\	
		\hline
	\end{tabular}
\end{table*}
